# Supplementary material for: Incommensurate magnetism in K$_2$MnS$_{2-x}$Se$_x$ and prospects for tunable frustration in a triangular lattice of pseudo-1D spin chains
Source: arXiv:1905.03318 source file (2019-05-08)
Supplement: Supplementary file 1 [file K2MnS2_supplemental.pdf]

**Incommensurate magnetism in $K_2MnS_{2-x}Se_x$ and prospects for tunable frustration in a triangular lattice of pseudo-1D spin chains**

Ankita Bhutani, Piush Behera, Rebecca D. McAuliffe, Huibo Cao, Ashfia Huq, Melanie J. Kirkham, Clarina dela Cruz, Toby Woods and Daniel P. Shoemaker

**Supplemental Material**

1 Figure, 1 Table

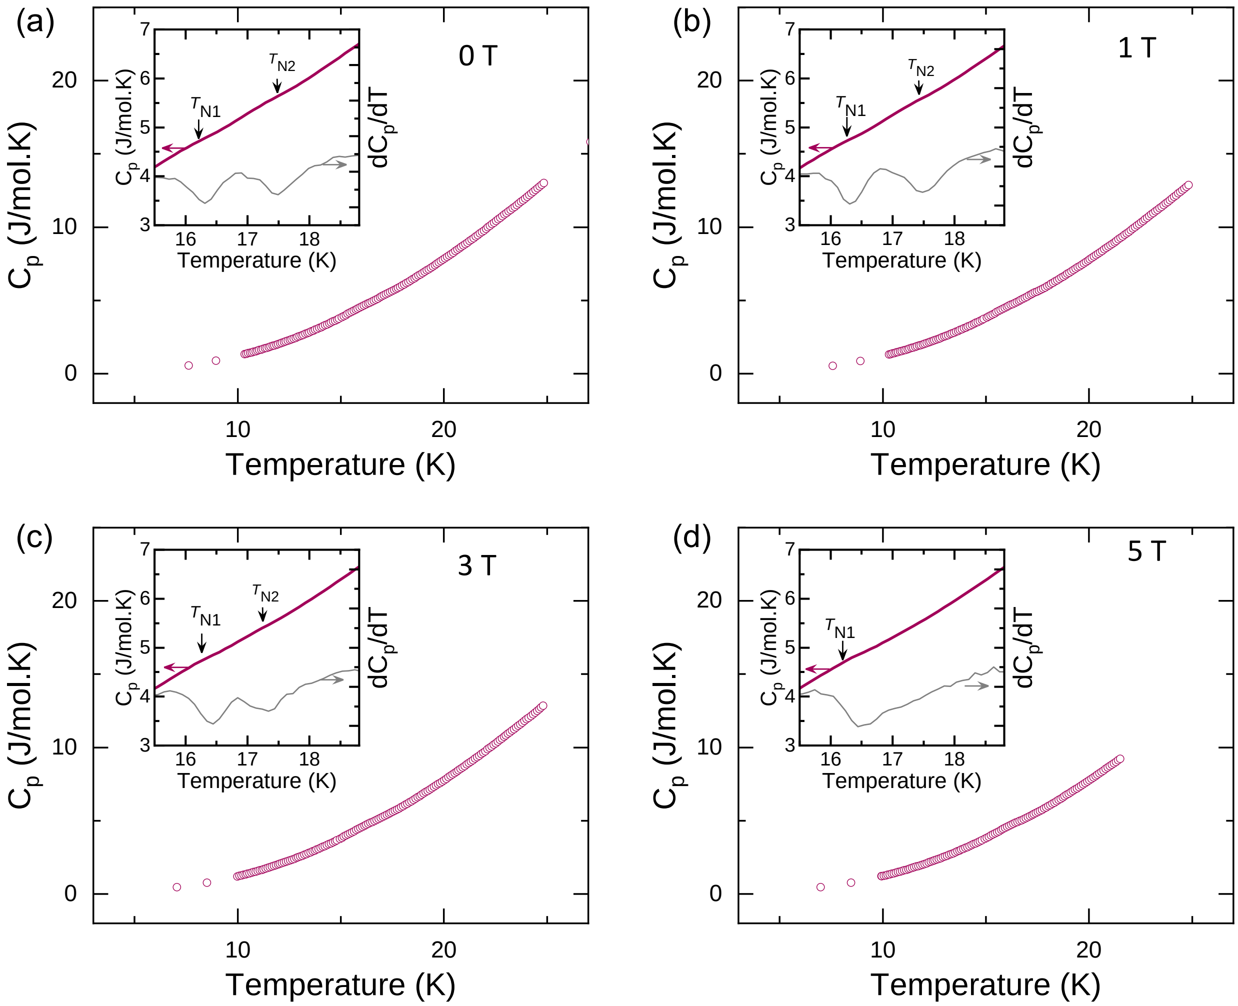


Figure S1. Heat capacity data for $K_2MnS_2$ at (a) 0 Tesla, (b) 1 Tesla, (c) 3 Tesla, and (d) 5 Tesla respectively, showing two closely-spaced transitions, that move closer together with increasing field and merge into 1 transition at 5 Tesla.

| Compound | ICSD# | M-M Dist. (Å) | Inter2 (Å) | Inter1 (Å) | Inter2/Inter1 |
|---|---|---|---|---|---|
| $Na_2ZnS_2$ | 33235 | 2.971 | 6.426 | 6.421 | 1.001 |
| $Na_2ZnS_2$ | 645008 | 2.971 | 6.426 | 6.421 | 1.001 |
| $K_2ZnO_2$ | 34603 | 2.701 | 6.030 | 5.967 | 1.011 |
| $Na_2CoS_2$ | 67386 | 2.925 | 6.447 | 6.373 | 1.012 |
| $Na_2FeS_2$ | 432210 | 2.815 | 6.546 | 6.435 | 1.017 |
| $Na_2CoSe_2$ | 624264 | 3.027 | 6.761 | 6.578 | 1.028 |
| $Na_2FeSe_2$ | 432211 | 2.928 | 6.807 | 6.608 | 1.030 |
| $Cs_2MnS_2$ | 65455 | 3.207 | 7.866 | 7.589 | 1.037 |
| $K_2MnS_2$ | 65453 | 3.090 | 7.206 | 6.932 | 1.040 |
| $K_2MnSe_2$ | 65456 | 3.220 | 7.507 | 7.166 | 1.048 |
| $Rb_2MnS_2$ | 65454 | 3.148 | 7.472 | 7.119 | 1.050 |
| $K_2CoS_2$ | 67387 | 3.043 | 7.090 | 6.710 | 1.057 |
| $K_2CoS_2$ | 623960 | 3.047 | 7.108 | 6.721 | 1.058 |
| $Rb_2MnSe_2$ | 65457 | 3.287 | 7.779 | 7.352 | 1.058 |
| $K_2CoS_2$ | 623958 | 3.035 | 7.079 | 6.681 | 1.060 |
| $Rb_2SnAs_2$ | 71223 | 3.471 | 7.919 | 7.454 | 1.062 |
| $K_2SiAs_2$ | 40426 | 3.170 | 7.440 | 6.999 | 1.063 |
| $Rb_2CoS_2$ | 67388 | 3.110 | 7.415 | 6.959 | 1.066 |
| $K_2SiP_2$ | 36367 | 3.054 | 7.318 | 6.867 | 1.066 |
| $K_2MnTe_2$ | 65459 | 3.437 | 7.982 | 7.478 | 1.067 |
| $K_2CoSe_2$ | 67390 | 3.195 | 7.432 | 6.960 | 1.068 |
| $Cs_2MnSe_2$ | 65458 | 3.342 | 8.105 | 7.589 | 1.068 |
| $K_2GeAs_2$ | 71222 | 3.274 | 7.518 | 7.028 | 1.070 |
| $Cs_2SiP_2$ | 71224 | 3.098 | 7.988 | 7.462 | 1.071 |
| $Rb_2SiAs_2$ | 60617 | 3.195 | 7.785 | 7.266 | 1.071 |
| $Cs_2SnAs_2$ | 71226 | 3.477 | 8.286 | 7.733 | 1.072 |
| $Cs_2CoS_2$ | 67389 | 3.161 | 7.756 | 7.232 | 1.072 |
| $Rb_2MnTe_2$ | 65460 | 3.498 | 8.233 | 7.667 | 1.074 |
| $Rb_2CoSe_2$ | 67391 | 3.236 | 7.684 | 7.155 | 1.074 |
| $Cs_2SiAs_2$ | 71225 | 3.210 | 8.146 | 7.571 | 1.076 |
| $Cs_2MnTe_2$ | 65461 | 3.570 | 8.579 | 7.963 | 1.077 |
| $Cs_2CoSe_2$ | 67392 | 3.292 | 8.020 | 7.429 | 1.079 |
| $K_2ZnTe_2$ | 420088 | 3.461 | 7.905 | 7.303 | 1.082 |

Table S1. Compounds in the structure type $K_2MnS_2$ (space group *Ibam*) with their Inorganic Crystal Structure Database identifier, metal-metal (M-M) separation distance, short and long interchain distances (Inter1 and Inter2), and anisotropy ratio Inter1/Inter2.
